# Supplementary material for: Rosetta Stone of Neural Mass Models
Source: arXiv:2512.10982 source file (2026-06-14)
Supplement: Supplementary file 1 [file appendix_kuramoto.tex]

In the main text, we begin with a pure phase oscillator model and gradually introduce increasing mathematical complexity.
Nonetheless, coupled phase oscillator models, particularly the Kuramoto model, were originally derived from arbitrary oscillator 
systems subject to weak perturbations by employing rigorous mathematical techniques.
Such approach, usually known as \emph{phase reduction}, was pioneered by Winfree and Kuramoto,
 and has been widely applied in mathematical neuroscience to capture the phase dynamics of both single-neuron and neural population models. For a comprehensive treatment of these methods, readers may refer to~\cite{Winfree2001,Kuramoto1984,hoppensteadt1997,Pikovsky2003}.
 Drawing on this literature, in this Appendix we provide a concise introduction to the phase reduction technique in a general setting, and then illustrate it using the Stuart–Landau oscillator, which naturally leads to the Kuramoto model.

\subsection{Phase of a perturbed oscillator}
\label{app:phase_of_perturbed_oscillator}
% PHASE OF A LIMIT-CYCLE
Let us consider an $m$-dimensional variable $\bs{x}\in\mathbb{R}^m$, whose time evolution is ruled by the differential equation
\begin{equation}\label{introeq:system}
\dot{\bs{x}}=\bs{\mathcal {F}}(\bs{x})
\end{equation}
where $\bs{\mathcal{F}}$ is a smooth function. Let us assume that equation~(\ref{introeq:system})
has an attracting limit-cycle with period $T$, $\bs {x}_{\text{LC}}(t)=\bs {x}_{\text{LC}}(t+T)$.
Thus, the curve $\bs{x}$ is, by definition, parameterized by time, $t\in[0,T)$.
We define the \emph{phase} of a point $\bs{x}(t)$ of $\bs x_{\text{LC}}$ as
\begin{equation}
\phi(\bs x(t)):=t\frac{2\pi}{T}\in[0,2\pi).
\end{equation}
For simplicity, we denote $\omega:=\frac{2\pi}{T}$.\\

% ISOCHRONES
The concept of phase is well defined for any point lying exactly on the limit cycle.
Nevertheless, the phase reduction approach is based on extending the notion of phase to a neighborhood $G\subset \mathbb{R}^m$ of $\bs x_{\text{LC}}(t)$.
Let $\bs y_0=\bs y(0)\in\mathbb{R}^m$ be a point in the state space close to, but not exactly on the periodic attractor $\bs x_{\text{LC}}$.
Since the limit cycle is stable, the trajectory $\bs y(t)$ will end up arbitrarily close to $\bs x_{\text{LC}}$ as $t\to\infty$,
thus will have a well defined phase, $\phi(\bs y(t))$.
Therefore, even if $\bs y_0$ is not on the invariant manifold,
one can find a point, $\bs x_0\in \bs x_{\text{LC}}$ such that, at long-term,
$\phi(\bs y(t))=\phi(\bs x(t))$.
One can then define the phase of $\bs y_0$ as $\phi(\bs y_0)=\phi(\bs x_0)$.
All the points in the neighborhood of $\bs x_{\text{LC}}$ associated to the same phase form a \emph{isochrone curve},
i.e., the isochrones are the level curves of the function $\phi$.
\\

This extension of the notion of phase to the vicinity of the periodic orbit preserves a constant time evolution:
\begin{equation}\label{introeq:phaseoscillator}
\dot \phi(\bs x)=\omega\;, \qquad \bs x \in G.
\end{equation}
Applying the chain rule and using Eq.~\ref{introeq:system}, one obtains
\begin{equation}
\dot \phi(\bs x)=\grad_{\bs x} \phi \cdot \bs{\mathcal{F}}(\bs x).
\end{equation}
Combining the two previous equations provides
\begin{equation}\label{introeq:phaseequality}
\grad_{\bs x} \phi \cdot \bs{\mathcal{F}}(\bs x)=\omega\;.
\end{equation}
This equation expresses then, that the variation of the phase under the effect of the field $\bs{\mathcal{F}}$
is constant.

% PHASE RESPONSE CURVE
We want to study oscillatory systems that are interacting with a certain environment, so, usually,
equation~(\ref{introeq:system}) is not enough for our purposes. One needs to
account for the effect that external perturbations have on the system.
Let us assume a perturbation on the evolution of $\bs x$, $\bs p(t)$, with a small amplitude parameter $ 0<\varepsilon \ll 1$,
\begin{equation}
 \dot{\bs{x}}=\bs{\mathcal {F}}(\bs{x})+\varepsilon \bs{p}(t).
\end{equation}
In order to keep arguing in terms of phases, one needs to find which is the impact of
such perturbation on the phase of the oscillator.
Applying again the chain rule to the time evolution of $\phi$, and using Eq.~(\ref{introeq:phaseequality}) one obtains
\begin{align}
\dot \phi(\bs x)
&=\grad_{\bs x}\phi \cdot \left(\bs{\mathcal{F}}(\bs x)+\varepsilon \bs p(t)\right) \\
&=\omega+\varepsilon \grad_{\bs x}\phi\cdot \bs p(t) \label{introeq:winfree}
\end{align}
Thus, as one would expect, the linear response of the phase $\phi$ to a perturbation of the trajectory is given by its gradient.
For this reason, the gradient of the phase along a certain unitary direction $\bs{\delta x}$ is usually referred to as the \emph{Phase Response Curve} (PRC), $Z(\phi):=\grad_{\bs { x}}\phi \cdot \bs {\delta x}$.
Following the definition of gradient, given a infinitesimal  perturbation $\varepsilon \bs{\delta x}$ of a point on the limit cycle $\bs x$,
 one can effectively compute the phase response curve as the normalized difference between the phase of $\bs {x}$,
 and that of $\bs{x}+\varepsilon \bs{\delta x}$,
\begin{equation}
Z(\phi)=\frac{ \phi(\bs x)-\phi(\bs{ x}+\varepsilon\bs{\delta x}) }{\varepsilon  }\;.
\end{equation}
Thus, a positive (resp. negative) PRC indicates that the perturbation has the effect of advancing (resp. delaying) the phase of the oscillator.
A zero PRC means that the perturbed point lies exactly on the isochrone of the original point.
For simplicity, on the following we assume that the perturbation $\bs p(t)$ has direction $\bs {\delta x}$ and modulus $p(t)$ so that
$\grad_{\bs x}\phi\cdot \bs p(t)=Z(\phi) p(t)$. Thus, Eq~(\ref{introeq:winfree}) now reads
\begin{equation}\label{introeq:winfree2}
\dot \phi(\bs x)=\omega + \varepsilon Z(\phi)p(t)\;.
\end{equation}
Systems with this form are known as \emph{Winfree-type models} of phase oscillators~\cite{Winfree2001},
where the PRC, $Z(\phi)$, and the shape of the forcing $\bs p(t)$ are defined independently one from the other.

\subsection{From Winfree to Kuramoto}

Let's assume now the phase dynamics of two interacting oscillators of Winfree type:
\begin{align}\label{introeq:winfree3}
\dot \phi_1 &= \omega_1 + \varepsilon Z(\phi_1)g(\phi_2)\\
\dot \phi_2 &= \omega_2 + \varepsilon Z(\phi_2)g(\phi_1)\;.
\end{align}
Notice that now the forcing term $p(t)$ has been replaced by a $2\pi$-periodic interaction function $g(\phi)$.
It is possible to further simplify this system by separating time scales on the dynamics of the phase model.
Since $\varepsilon\ll 1$ in Eq.~(\ref{introeq:winfree3}), one expects that the changes
in the evolution of $\phi_j$ mostly happen at a slow time scale, since the fast dynamics is
driven by the natural frequency of oscillation $\omega_j$.
Let's study then the time evolution of the slow variables $\varphi_j=\phi_j-\omega_j t$.
With this change of variables, equation~(\ref{introeq:winfree3}) now reads
\begin{equation}
\dot \varphi_j=   \varepsilon Z(\varphi_j-\omega_j t)g(\varphi_k-\omega_k t)\;.
\end{equation}
In order to retain the terms relevant for the evolution of $\varphi_j$ one can expand
the previous equation in Fourier series,
\begin{align}\label{introeq:tokuramoto}
\dot \varphi_j=   \varepsilon  Z(\varphi_j-\omega_j t)g(\varphi_k-\omega_k t)
        &=\frac{\varepsilon}{4\pi^2}\sum_{m,n}\tilde Z(m)\tilde p(n)e^{-i[m(\varphi_j-\omega_j t) +n(\varphi_k-\omega_k t)]}\\
        &=\frac{\varepsilon}{4\pi^2}\sum_{m,n}\tilde Z(m)\tilde p(n)e^{-im(\varphi_j-\varphi_k)}e^{i(m\omega_j + n\omega_k)t}\;.
\end{align}
The last expression provides a separation of the fast and slow terms in the series:
the terms with
\begin{equation}
 m\omega_j +n \omega_k \simeq 0
\end{equation}
are resonant, and, therefore, lead to slow dynamics.
The other terms, instead, have explicit dependence on $t$, and, therefore, lead to rapid changes.
Thus, in order to keep only the relevant dynamics of the system, one can average out
the non-resonant terms.
Under the assumption that the natural frequencies of the two oscillator are comparable, \emph{i.e.}, $\omega_j\simeq \omega_k$,
the terms of Eq.~(\ref{introeq:tokuramoto}) relevant for the dynamics are those with
$m=-n$.
This leads to
\begin{equation}
    \dot \varphi_j=   
         =\frac{\varepsilon}{4\pi^2}\sum_{n=-\infty}^\infty\tilde Z(-n)\tilde p(n)e^{-in(\varphi_k-\varphi_j)}=H(\varphi_j-\varphi_k) 
\end{equation}
where the \emph{coupling function} $H$ can be computed as
\begin{equation}
H(\psi):=\frac{1}{4\pi^2}\sum_{n=-\infty}^\infty \tilde Z(-n)\tilde p(-n)e^{-in \psi}
=\frac{1}{2\pi}\int_0^{2\pi} Z(t)p(t+\psi) dt.
\end{equation}
Writing now system~(\ref{introeq:winfree3}) into the original variables, we finally obtain:
\begin{align}\label{introeq:phasemodel}
\dot \phi_1&=\omega_1+\varepsilon H(\phi_2 -\phi_1)\\
\dot \phi_2&=\omega_2+\varepsilon H(\phi_1 -\phi_2)\;.
\end{align}
Phase oscillators ruled by equations of this type are known as \emph{Kuramoto-Daido type} models.
Despite their simplicity, such systems provide a good framework
to study emerging phenomena on networks of oscillators.
The simplest of these models corresponds to $H$ being composed of a single harmonic, i.e.,
$$H(\psi) = \sin(\psi-\alpha),$$
leading to the famous Kuramoto-Sakaguchi model. 
Nonetheless, the phase reduction of most nonlinear oscillators contain more harmonics in their 
coupling function, which usually also increase the complexity of the model dynamics.

Here, we provided a simple intuitive arguments on how the time-scale separation is being performed.
Formally, the coupling function $H$ emerges from applying averaging theory to system \eqref{introeq:winfree3}.
% COMMENT ON "ORDER EPSILON" AND "HIGHER ORDER INTERACTIONS".
These rigorous derivations also allow to extend this approach to more complex situations, including
an arbitrary number of oscillators, 
cases in which the interaction function $g$ depends on both, pre and post-synaptic units, $g(\phi_1,\phi_2)$,
and cases with other resonant relation between the units. 
Nonetheless, here we want to emphasize the two main assumptions that allow to obtain Kuramoto-Daido models
from arbitrary limit cycles: weak coupling ($\varepsilon\ll 1$), and weak frequency heterogeneities ($\omega_1\approx \omega_2$). 

\subsection{Phase reduction of a Stuart-Landau system}

In general, performing the phase reduction of a nonlinear oscillator requires a numerical approach.
Due to its simplicity and symmetry properties, the Stuart-Landau oscillator is a notable exception.
Here we reproduce a well-known result that a system of coupled Stuart-Landau oscillators
leads to the Kuramoto-Sakaguchi model:
\begin{equation}
\dot{z}_{i} = (\alpha + i\,\omega_{i})\,z_{i}
             - (\gamma + i\,\beta)\,\lvert z_{i}\rvert^{2}z_{i}
             + \frac{\varepsilon}{N}\sum_{j=1}^{N}\bigl(z_{j}-z_{i}\bigr)\;.
\end{equation}

Let's first determine the phase variable of an uncoupled oscillator.
We work using the polar representation:
\begin{align}
  \dot{r}      &= \alpha\,r \;-\; \gamma\,r^{3},\\
  \dot{\theta} &= \omega \;-\; \beta\,r^{2}.
\end{align}
The system contains an (unstable) fixed point at $r=0$.
For any other initial condition, $r(0)=r_0\neq 0$ and $\theta(0)=\theta_0$, the solution of the system reads:
\begin{equation}
    r(t) = \sqrt{\frac{\alpha}{\gamma + \left(\frac{\alpha}{r_0^2}-\gamma\right)e^{-2\alpha t}}}
    \qquad
    \theta(t) = \omega - \frac{\alpha\beta}{\gamma} +\theta_0 
    - \frac{\beta}{2\gamma} \ln\left[ \frac{\gamma}{\alpha} r_0^2 + e^{-2\alpha t}\left(1-\frac{\gamma}{\alpha}r_0^2 \right)\right]\;. 
\end{equation}
As $t\to\infty$ the equation evolves towards a limit cycle with amplitude $r_* = \sqrt{\alpha/\gamma}$ and frequency 
$\Omega = \omega - \frac{\alpha\beta}{\gamma}$.
If  the system is initialized exactly at the limit-cycle, then the phase is simply $\phi(r,\theta) = \theta$.
For initial conditions outside the invariant manifold, the system converges to the limit cycle with phase
$$\phi(r,\theta) = \theta - \frac{\beta}{2\gamma}\ln\left(\frac{\gamma}{\alpha} r_0^2 \right).$$
From this explicit expression we can observe the isochrones of the Stuart-Landau oscillator are given by
setting $\phi = k$, where $k\in[0,2\pi)$ is constant.
We can also check that this definition of phase produces a uniform rotation from Eq.~\eqref{introeq:phaseequality}:
 $$\nabla \phi(r,\theta)\cdot \bs{\mathcal{F}} = \omega - \frac{\alpha \beta }{\gamma}.$$

Let's consider now the perturbed system:
\begin{equation}
\dot{z}_{i} = (\alpha + i\,\omega_{i})\,z_{i}
             - (\gamma + i\,\beta)\,\lvert z_{i}\rvert^{2}z_{i}
             + {\varepsilon} \delta z.
\end{equation}
As explained before, the PRC of the system can be computed as the phase gradient at a given perturbation direction,
in this case
$$Z(\phi)=\grad_{\bs z}\phi\cdot \delta z.$$
For simplicity, we proceed in Cartesian coordinates:
\begin{equation}
    \phi(x,y) = \arctan\left(\frac{y}{x}\right) - \frac{\beta}{2\gamma}\ln\left(\frac{\gamma}{\alpha} (x^2+y^2) \right)
\end{equation}
thus
\begin{align}
\grad_{\bs z}\phi &= \left( \frac{-1}{x^2+y^2}\left(\frac{\beta}{\gamma}x+y\right), \frac{1}{x^2+y^2}\left(x-\frac{\beta}{\gamma}y\right)\right) \\
&= \frac{1}{\sqrt{\alpha}} \left( - \beta\cos(\phi)-\gamma\sin(\phi), \gamma \cos(\phi)-\beta \sin(\phi) \right).
\end{align}
Therefore, the phase dynamics of a single, weakly perturbed Stuart-Landau oscillator
are given by
$$\dot \phi = \Omega + \frac{\varepsilon}{\sqrt{\alpha}}
\left[ 
\left( - \beta\cos(\phi)-\gamma\sin(\phi)\right)\delta x
\left(\gamma \cos(\phi)-\beta \sin(\phi) \right)\delta y
\right] $$
where $\delta z = (\delta x,\delta y)$.
In the coupled system, the perturbation comes from the other oscillators of the network, and thus chages in time.
In particular 
\begin{align}
\delta x_i &= \frac{1}{N}\sum_{j=1}^N (x_j-x_i) = \frac{1}{N}\sqrt{\frac{\alpha}{\gamma}}\sum_{j=1}^N (\cos(\phi_j)-\cos(\phi_i))\\
\delta y_i &= \frac{1}{N}\sum_{j=1}^N (y_j-y_i) = \frac{1}{N}\sqrt{\frac{\alpha}{\gamma}}\sum_{j=1}^N (\sin(\phi_j)-\sin(\phi_i)) . 
\end{align}
Inserting these expressions into the PRC and simplifying the terms using trigonometric identities, we finally obtain
\begin{equation}
    \phi_i = \Omega_i + \varepsilon K \frac{\beta}{\gamma}  + \varepsilon \frac{K}{N}\sum_{j=1}^N \sin(\phi_j-\phi_i-\alpha)
\end{equation}
where 
$$\Omega_i =  \omega_i - \frac{\alpha \beta }{\gamma},\quad K = \sqrt{1+\frac{\beta^2}{\gamma^2}},\quad\text{and}\quad\alpha=\arctan\left(\frac{\beta}{\gamma} \right).$$
In this case, no averaging is needed to obtain a Kuramoto-Daido type of model,
since we have already obtained a coupling function that depends only on the phase differences.
Moreover, the coupling is given by a single harmonic, thus ultimately providing a Kuramoto-Sakaguchi model. 
We emphasize, again, that this is specific for the Stuart-Landau oscillator, and other models can lead to 
coupling functions with several harmonics.
